# Supplementary material for: P3HT-Fullerene Blends: a Classical Molecular Dynamics Simulation
Source: arXiv:1805.10335 ancillary file (2018-05-25)
Supplement: Supplementary file 1 [file T_NFF_arxiv_sup.pdf]

# P3HT-Fullerene Blends: a Classical Molecular Dynamics Simulation Supplementary Information

Rodrigo Ramos† and Marilia J. Caldas*,¶

†*Instituto de Física, Universidade de São Paulo, 05508-900 São Paulo, SP, Brazil*

‡*Now at: Centro Universitário das Faculdades Metropolitanas Unidas, São Paulo, SP, Brazil*

¶*Instituto de Física, Universidade de São Paulo, São Paulo, SP, Brazil*

E-mail: mjcaldas@usp.br

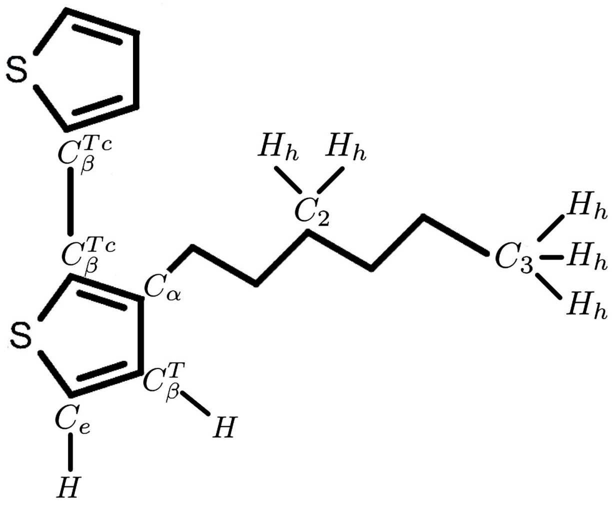


Figure 1: Atomic types for 3(hexyl-thiophene) units, defined by the first neighbor connections.

The partial charges (in electron units $e$) listed in table 1 are averages of the values, obtained from Hirshfeld partitioning with PBE-DFT through the FHI-aims code, for the chosen

molecules: thiophene monomer T1, 3-hexyl-thiophene monomer 3HT1, bi- ter- and tetra 3-hexyl-thiophene oligomers 3HT2, 3HT3 and 3HT4; infinite 3HT regioregular polymers with planar P3HT-*pl* (local minimum configuration) and normal dihedral-angle P3HT. The resulting average values obey charge neutrality constraint for each system (or segment), obtained by adding (or subtracting) charge to each atom, weighted by the preassigned charges, in order to avoid eventual nonzero total charge inside the system unit cell. The atomic types are illustrated in figure 1. The crystalline structures adopted for the parametrization procedure are illustrated in figures 2-4.

Table 1: Atomic types, charges (ATC, electron units $e$) and respective non-bonded interaction coefficients for Lennard-Jones potential developed in this work, according to the Tkatcenko-Scheffler[1] procedure, for hexyltiophenes. In the case of fullerene we keep the original UFF $r_0 = 3.85$ Å, while D is reduced to 0.0698 kcal/mol., following the same procedure.

| Atom type | q (e) | $r_0$ (Å) | D (kcal/mol) |
|---|---|---|---|
| S | 0.110 | 4.035 | 0.379 |
| $C_e$ | -0.900 | 3.975 | 0.051 |
| $C_\beta^{Tc}$ | -0.040 | 3.975 | 0.051 |
| $C_\beta^{T}$ | -0.080 | 3.975 | 0.051 |
| $C_\alpha$ | 0.000 | 3.850 | 0.070 |
| $C_2$ | -0.070 | 4.350 | 0.030 |
| $C_3$ | -0.105 | 4.350 | 0.030 |
| $H_h$ | 0.035 | 2.830 | 0.030 |
| $H$ | 0.050 | 2.830 | 0.030 |

The dihedral torsion angle for thiophene chains is fitted in the displaced-dihedral form shown in equation 1 for the torsional component of the total energy curve calculated[2] for T4, employing the MP2 method:

$$U^d(\phi_{ijkl}) = \sum_{n=1}^{4} \frac{1}{2} U_{ijkl}(n) \left[1 + \cos(n\phi_{ijkl} + \phi_{ijkl}^{(0)})\right] \quad (1)$$

where $i, j, k, l$ refer to the atom types in figure 1 (in the unsubstituted T4 molecule, the $C_\alpha$ type is not present, there are two $C_\beta^T$), and the $U_{ijk}$ parameters are given in table 2.

For the phase $\phi^{(0)}$, the ordering for $ijkl$ with $n$ in the table is $a: S - C_\beta^{Tc} - C_\beta^{Tc} - S$; $b: S - C_\beta^{Tc} - C_\beta^{Tc} - C_\beta^{T}$; $c: C_\beta^{T} - C_\beta^{Tc} - C_\beta^{Tc} - C_\beta^{T}$.

Table 2: Obtained parameters $U^d(\phi_{ijkl})$ (in kcal/mol) for the thiophene oligomer T4, with $\phi_{ijkl}^{(0)}$ as described in the text.

| $n$ | $U_{ijk}$ | $\phi^{(0)}(a)$ | $\phi^{(0)}(b)$ | $\phi^{(0)}(c)$ |
|---|---|---|---|---|
| 1 | 0.7117 | 0 | $\pi$ | 0 |
| 2 | -1.5414 | 0 | 0 | 0 |
| 3 | -0.1764 | 0 | $\pi$ | 0 |
| 4 | 0.6670 | 0 | 0 | 0 |

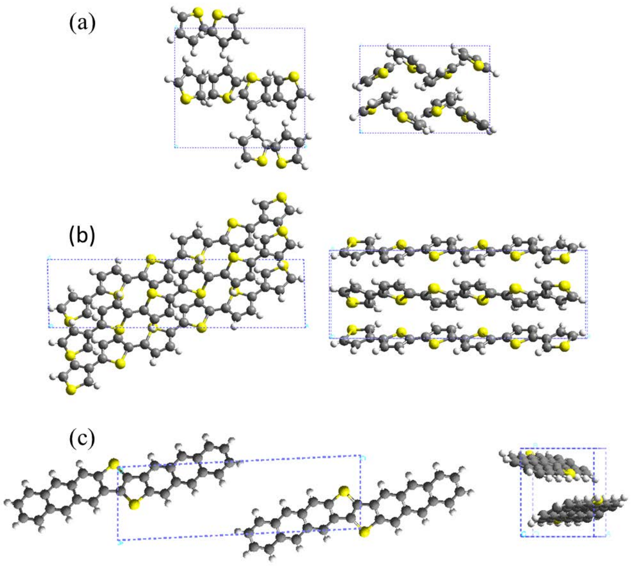


Figure 2: Molecular crystals used for NanomolFF parametrization: (a) Thiophene T1; (b) Sexithiophene T6; (c) Dianthra[2,3-b:2',3'-f]thieno[3,2-b]thiophene Di-AntT.

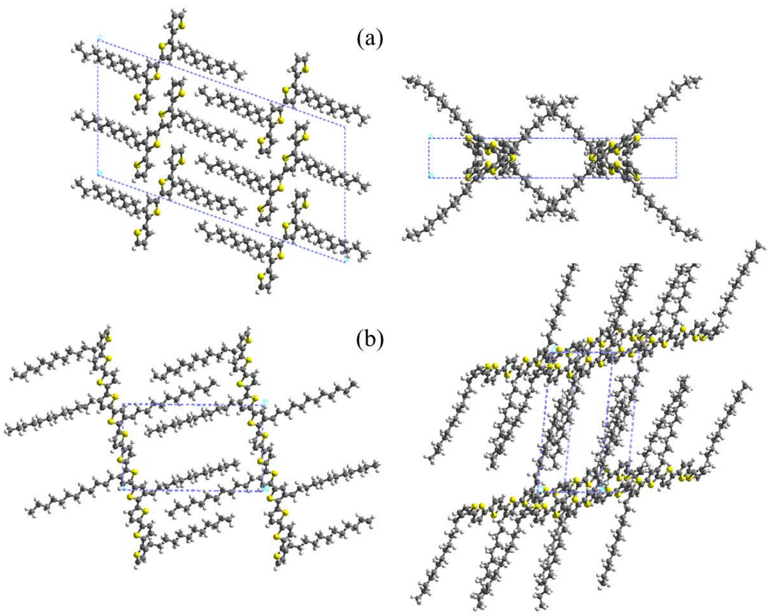


Figure 3: Molecular crystals used for NanomolFF parametrization: (a) Bi-(thiophene-decylthiophene) Bi-T3DT; (b) tetra-(thiophene-decylthiophene) Tetra-T3DT.

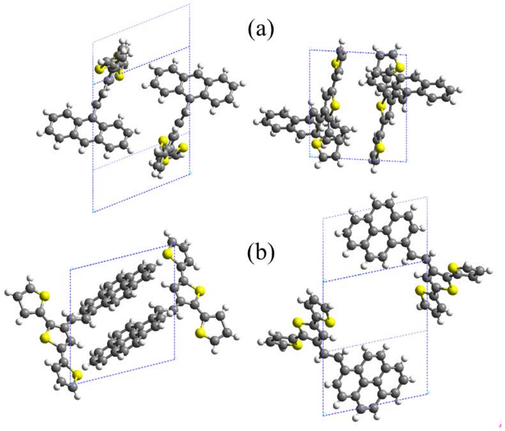


Figure 4: Molecular crystals used for NanomolFF parametrization: (a) terthiophene-anthracene T3-Ant; (b) terthiophene-pyrene 3T-Pyr. Here we have also acene-based molecules, and we used the ATCs obtained for the thiophene set described above, so we applied charge neutrality for the cell optimization.

# References

(1) Tkatchenko, A.; Scheffler, M. Phys. Rev. Lett. **2009**, 102, 073005.

(2) Alves-Santos, M.; Caldas, M. J. Synth. Met. **2009**, 159, 2302 – 2305.

(3) NIST, Chemistry Webbook – http:webbook.nist.govchemistry.

Table 3: Molecular crystals used for NanomolFF parametrization: Lattice parameters.[3]

| Latt. Const. Å | Crystal | Exp | NFF | Dev. (%) | Angle Deg. | Exp | NFF | Dev. (%) |
|---|---|---|---|---|---|---|---|---|
| ***a*** | T1 A | 11.02 | 11.13 | 0.97 | $\alpha$ | 90 | 90 | 0.00 |
| | T1 B | 11.05 | 11.13 | 0.68 | | 90 | 90 | 0.00 |
| | T6 A | 22.45 | 22.54 | 0.41 | | 90 | 90 | 0.00 |
| | T6 B | 7.61 | 7.22 | 5.08 | | 90 | 90 | 0.00 |
| | Di-AntT | 6.26 | 6.62 | 5.82 | | 90 | 90 | 0.00 |
| | Bi-T3DT | 36.15 | 34.95 | 3.32 | | 90 | 90 | 0.00 |
| | Tetra-T3DT | 9.62 | 9.70 | 0.81 | | 87.83 | 88.16 | 0.33 |
| | T3-Ant A | 9.11 | 9.17 | 0.71 | | 90 | 90 | 0.00 |
| | T3-Ant B | 9.24 | 9.17 | 0.74 | | 90 | 90 | 0.00 |
| | 3T-Pyr A | 9.74 | 10.67 | 9.59 | | 61.24 | 64.36 | 3.12 |
| | 3T-Pyr B | 9.77 | 10.06 | 2.97 | | 68.42 | 68.02 | 0.40 |
| ***b*** | T1 A | 7.43 | 7.37 | 0.82 | $\beta$ | 90 | 90 | 0.00 |
| | T1 B | 7.50 | 7.37 | 1.79 | | 90 | 90 | 0.00 |
| | T6 A | 7.72 | 7.27 | 5.78 | | 90 | 90 | 0.00 |
| | T6 B | 41.91 | 42.50 | 1.41 | | 90 | 90 | 0.00 |
| | Di-AntT | 7.57 | 7.13 | 5.87 | | 90 | 90 | 0.00 |
| | Bi-T3DT | 5.47 | 5.42 | 0.95 | | 90 | 90 | 0.00 |
| | Tetra-T3DT | 13.90 | 13.98 | 0.64 | | 87.83 | 88.16 | 0.33 |
| | T3-Ant A | 5.73 | 5.73 | 0.00 | | 90 | 90 | 0.00 |
| | T3-Ant B | 5.72 | 5.73 | 0.17 | | 90 | 90 | 0.00 |
| | 3T-Pyr A | 11.71 | 10.67 | 8.90 | | 61.24 | 64.36 | 3.12 |
| | 3T-Pyr B | 10.80 | 11.58 | 7.24 | | 68.42 | 68.02 | 0.40 |
| ***c*** | T1 A | 10.10 | 10.19 | 0.92 | $\gamma$ | 90 | 90 | 0.00 |
| | T1 B | 10.16 | 10.19 | 0.28 | | 90 | 90 | 0.00 |
| | T6 A | 5.99 | 6.29 | 4.92 | | 90 | 90 | 0.00 |
| | T6 B | 11.03 | 11.37 | 3.04 | | 90 | 90 | 0.00 |
| | Di-AntT | 20.83 | 20.47 | 1.73 | | 90 | 90 | 0.00 |
| | Bi-T3DT | 18.67 | 19.33 | 3.54 | | 90 | 90 | 0.00 |
| | Tetra-T3DT | 21.70 | 21.31 | 1.77 | | 72.9 | 72.0 | 0.90 |
| | T3-Ant A | 18.16 | 17.79 | 2.03 | | 90 | 90 | 0.00 |
| | T3-Ant B | 18.21 | 17.79 | 2.29 | | 90 | 90 | 0.00 |
| | 3T-Pyr A | 11.85 | 11.84 | 0.02 | | 72.31 | 74.99 | 2.68 |
| | 3T-Pyr B | 12.03 | 11.84 | 1.55 | | 84.84 | 92.94 | 8.10 |
